# Supplementary material for: Modeling Heat Dissipation at the Nanoscale: An Embedding Approach for Chemical Reaction Dynamics on Metal Surfaces
Source: arXiv:1402.5831 source file (2014-05-13)
Supplement: Supplementary file 1 [file QMMe-SupportingInformation.pdf]

published in *Angew. Chem. Int. Ed.* **2014**, *53*, 4721–4724, DOI: 10.1002/anie.201400066

# Modeling Heat Dissipation at the Nanoscale: An Embedding Approach for Chemical Reaction Dynamics on Metal Surfaces

## *Supporting Information: Technical Details*

Jörg Meyer* and Karsten Reuter

Lehrstuhl für Theoretische Chemie, Technische Universität München,

Lichtenbergstraße 4, D-85748 Garching, Germany,

http://www.th4.ch.tum.de

May 13, 2014

*joerg.meyer@ch.tum.de

*present address:* Leiden Institute of Chemistry, Gorlaeus Laboratories, Leiden University, P.O. Box 9502, 2300 RA Leiden, The Netherlands

published in *Angew. Chem. Int. Ed.* **2014**, *53*, 4721–4724, DOI: 10.1002/anie.201400066

# 1 Technical Details – Overview

We have extended the LAMMPS package[1] to generate molecular dynamics (MD) trajectories according to the QM/Me embedding scheme according to

$$V^{\text{QM/Me}}(R) = V^{\text{Me}}(R_{\text{bath}}) + \underbrace{\left[E^{\overline{\text{QM}}}(R_{\text{slab}} \cup R_{\text{ads}}) - E^{\overline{\text{QM}}}(R_{\text{slab}})\right]}_{V^{\Delta\overline{\text{QM}}}(R_{\text{slab}} \cup R_{\text{ads}})} . \tag{1}$$

as proposed in the main article. In order to obtain the forces $\mathbf{F}_I^{\Delta\overline{\text{QM}}} = -\nabla_{\mathbf{R}_I} V^{\Delta\overline{\text{QM}}}$ during each time step of $\Delta t = 2.5$ fs, two DFT supercell calculations for the embedding cell with 72 Pd atoms depicted in Figure 1 (see main article) are carried out with the CASTEP code,[2] which we describe in more detail in Section 2. $V^{\text{Me}}$ describes a cubic bath of 125,000 atoms employing a classical interatomic potential (CIP) according to the modified embedded atom method (MEAM),[3] we have reparameterized as detailed in Section 3 to seamlessly fit the DFT data within LAMMPS. Finally, in Section 4 we present further technical details of the employed MD simulation setup and discuss some important aspects related to the embedding scheme itself.

# 2 DFT calculations

The embedding cells used here for the periodic boundary conditions supercell DFT calculations consist of 3-layer slabs, which are $8 \times 3$ multiples of the Pd(100) surface unit cell, separated by a vacuum distance of at least 15 Å. The surface Brillouin has been sampled by a $2 \times 4 \times 1$ Monkhorst-Pack **k**-point grid[4] and using a (first order) Methfessel-Paxton broadening[5] with a width of 0.1 eV. The exchange-correlation functional due to Perdew, Burke and Ernzerhof (PBE)[6] is employed. Corresponding ultrasoft pseudopotentials from the CASTEP[2] default library were used to describe the palladium and oxygen atoms together with a plane wave cut-off of 400 eV, and thorough convergence tests based on oxygen adsorption energies have been performed.[7] Since the initial conditions

| | $E_0$ | $R_0$ | $\alpha$ | $A$ | $\beta^{(0)}$ | $\beta^{(1)}$ | $\beta^{(2)}$ | $\beta^{(3)}$ | $t^{(0)}$ | $t^{(1)}$ | $t^{(2)}$ | $t^{(3)}$ |
|---|---|---|---|---|---|---|---|---|---|---|---|---|
| Baskes[3] | 3.91 | 2.75 | 6.43 | 1.01 | 4.98 | 2.2 | 6.0 | 2.2 | 1.0 | 2.34 | 1.34 | 4.48 |
| Beurden[12] | 3.68 | 2.80 | 6.24 | 1.0 | 5.28 | 4.07 | 4.93 | 2.18 | 1.0 | 2.27 | 6.22 | 3.68 |
| MEAMopt | 3.88 | 2.78 | 6.18 | 1.0 | 4.30 | 4.77 | 0.89 | 0.0 | 1.0 | 8.68 | 5.11 | −10.93 |

***Table 1:*** Parameters for the optimized MEAM potential (MEAMopt) obtained in this work by force matching DFT data as described in the text. The cohesive energy $E_0$ (eV), as well as the nearest neighbor distance $R_0$ (Å) are taken directly from the DFT calculations. This also holds for the dimensionless parameter $\alpha = \sqrt{\frac{9BR_0^3}{4E_0}}$ with the help of the bulk modulus $B$ obtained from the latter. The scaling parameter $A$ has been kept fixed at 1.0. The remaining 8 dimensionless $\beta^{(i)}, t^{(i)}, i \in \{0,1,2,3\}$ have then been determined by a force matching procedure as detailed in the text. Values from Baskes[3] as well as van Beurden and Kramer[12] are given for reference.

| | $d_{12}$ [Å] | $d_{23}$ [Å] | $d_{34}$ [Å] |
|---|---|---|---|
| CASTEP | 1.948 | 1.970 | 1.965 |
| MEAMopt | 1.943 | 1.968 | 1.964 |

***Table 2:*** Comparison of interlayer distances $d_{ij}$ between layers $i$ and $j$ of the Pd(100) surface obtained from DFT-PBE (CASTEP) and the optimized MEAM potential (MEAMopt).

obtained from the frozen-surface statistical sampling[7] are close enough to the surface for the initial gas-phase triplet state of $O_2$ to have already been quenched,[8] the calculations are carried out without spin-polarization. Using these settings identically for both DFT calculations required at each time step during the QM/Me-based dynamics ensures a numerically well-defined construction of $V^{\Delta\overline{\mathrm{QM}}}(R_{\mathrm{slab}})$. Convergence of the electronic self-consistency cycles proves difficult for the present system, and thus the tight criteria ($\leq 0.5 \cdot 10^{-3}$ eV A$^{-1}$ for the forces corresponding to a total energy convergence of about $\leq 10^{-8}$ eV)) can only be satisfied along entire trajectories by switching to CASTEP's ensemble DFT-based electronic minimization[9] dynamically when required.[7] In the present context, this is of particular relevance to avoid "artificial energy dissipation" due to well-known total energy drifts in *ab initio* molecular dynamics which are caused by insufficient numerical force convergence.[10,11]

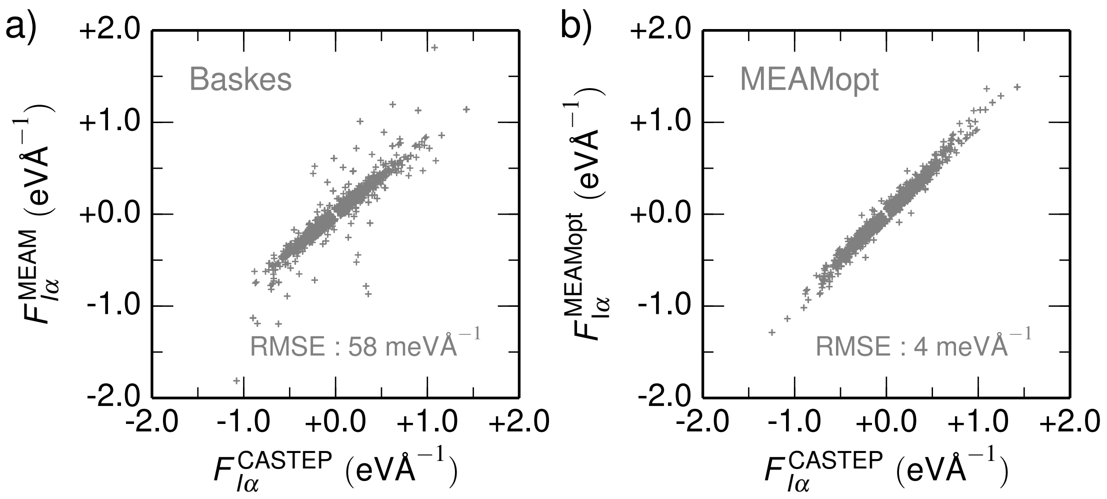


***Figure 1:*** Force errors a) before and b) after optimization of the MEAM potential by force matching. The former is based on the (original) parametrization by Baskes[3] to empirical data, which is given together with the one constituting MEAMopt in Table 1.

# 3 MEAM potential

MEAM potentials have been considered for $V^{\text{Me}}$ in this work because they are based on a small number of parameters, enabling a convenient reparametrization that seamlessly fits the quantum mechanical description. The parameters include the (fcc) bulk nearest neighbor distance $R_0$, cohesive energy $E_0$ and bulk modulus $B$ (determining $\alpha = \sqrt{\frac{9BR_0^3}{4E_0}}$), which have all been obtained directly within the DFT setup described above. The remaining ones ($\beta^{(i)}, t^{(i)}, i \in \{0,1,2,3\}$) are obtained by force matching[13] to a database of more than 8000 thousand DFT force components from several snapshots of Pd slab calculations analogue to those providing $E^{\overline{\text{QM}}}(R_{\text{slab}})$ in QM/Me trajectories, employing existing parametrizations[3,12] as a starting point. The parameters of the best fit (MEAMopt) are given in Table 1. Using the same notation as in the work by Valone *et al.*,[14] the reader is referred to that work for more details and references to the modified embedded atom method. The present MEAMopt reparametrization features a root mean square error of 4 meVÅ$^{-1}$ (cf. Figure 1), mimics the minute layer relaxations of the Pd(100) surface (as given by PBE-DFT) within less than 0.01 Å (cf. Table 2) and yields a surface phonon spectrum in excellent agreement with the latter (cf. Figure 2). Further details will be included in a forthcoming publication and can

published in *Angew. Chem. Int. Ed.* **2014**, *53*, 4721–4724, DOI: 10.1002/anie.201400066

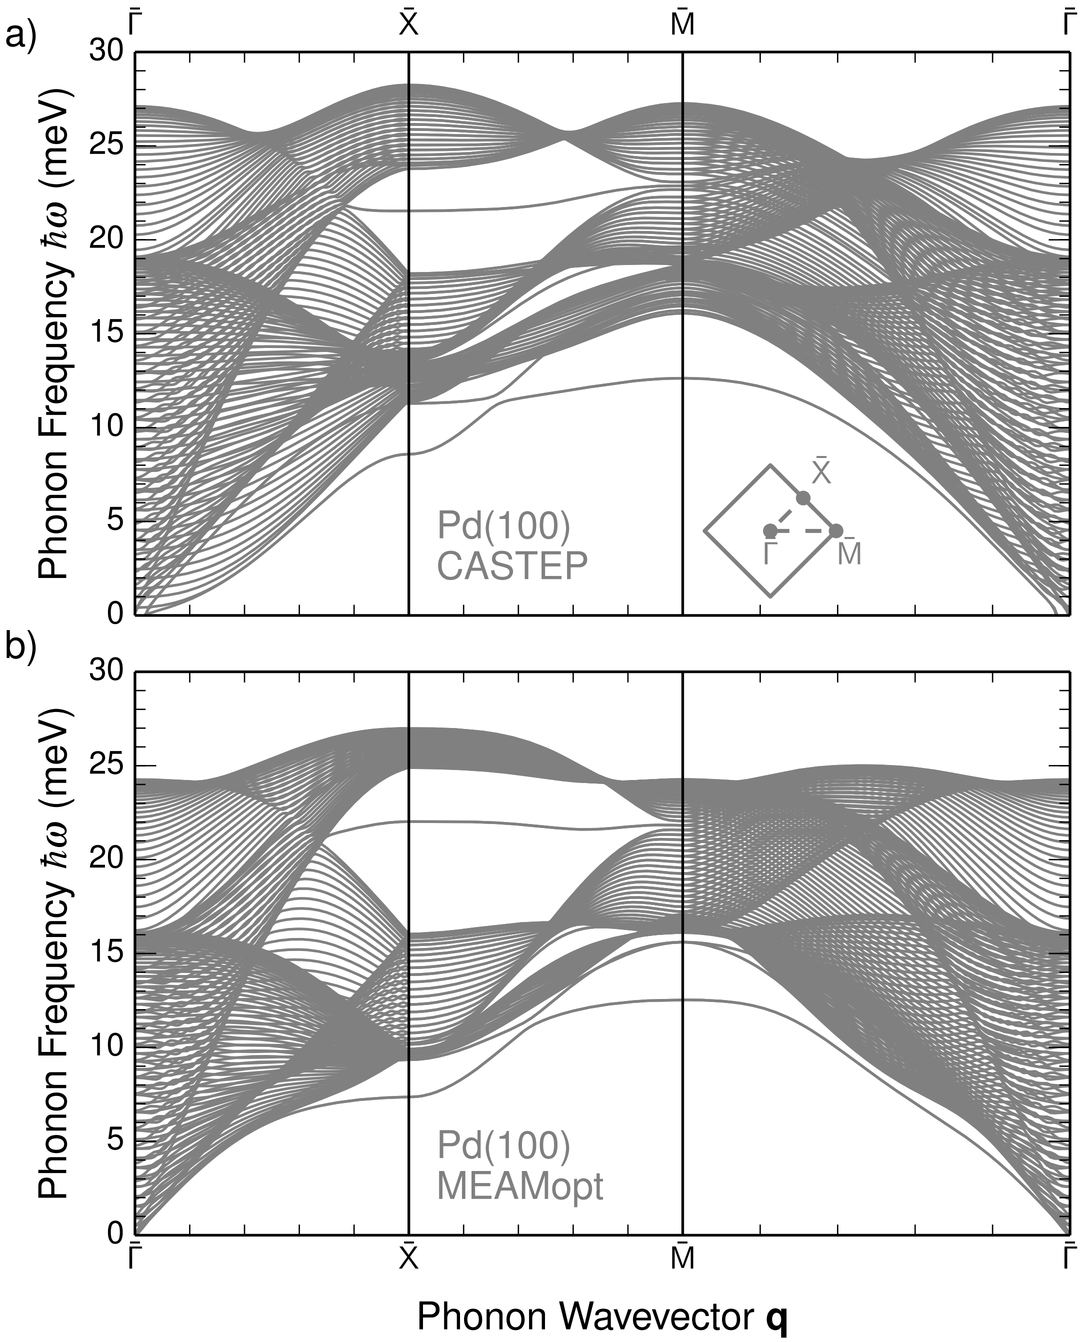


***Figure 2:*** Surface phonon dispersion of Pd(100) as obtained by a) DFT-PBE (CASTEP) and b) the optimized MEAM potential (MEAMopt).

be found in[7] for now. We finally note that future QM/Me applications might benefit from recent more sophisticated adaptions of modern classical interatomic potentials[15,16] for the description of the bath of metal atoms. These are still several orders of magnitude less expensive than (currently impossible) modeling of the entire bath by DFT.[17]

# 4 QM/Me embedding

Forces obtained from $V^{\text{QM/Me}}$ (cf Equation (1)) are given by

$$\mathbf{F}_I^{\text{QM/Me}}(R) = \mathbf{F}_I^{\text{Me}}(R_{\text{bath}}) \; + \; \mathbf{F}_I^{\Delta\overline{\text{QM}}}(R_{\text{slab}} \cup R_{\text{ads}}) \quad \text{with } I \in \text{model}\,, \tag{2}$$

where the individual contributions are

$$\mathbf{F}_I^{\text{Me}}(R_{\text{bath}}) = \begin{cases} -\nabla_{\mathbf{R}_I} V^{\text{Me}}(R_{\text{bath}}) & \text{if } I \in \{\text{bath}\} \\ 0 & \text{otherwise} \end{cases} \tag{3a}$$

and

$$\mathbf{F}_I^{\Delta\overline{\text{QM}}}(R_{\text{slab}} \cup R_{\text{ads}}) = \begin{cases} -\nabla_{\mathbf{R}_I} E^{\overline{\text{QM}}}(R_{\text{slab}} \cup R_{\text{ads}}) & \text{if } I \in \{\text{adsorbate atoms}\} \\ -\Big[\nabla_{\mathbf{R}_I} E^{\overline{\text{QM}}}(R_{\text{slab}} \cup R_{\text{ads}}) \\ \qquad -\nabla_{\mathbf{R}_I} E^{\overline{\text{QM}}}(R_{\text{slab}})\Big] & \text{if } I \in \{\text{metal atoms in embedding cell}\} \\ 0 & \text{otherwise} \end{cases} \tag{3b}$$

Within this supporting material we provide an extension package `fix_ext_forces` for the classical MD code LAMMPS,[1] which allows to evaluate $-\nabla_{\mathbf{R}_I} E^{\overline{\text{QM}}}(R_{\text{slab}} \cup R_{\text{ads}})$ and $-\nabla_{\mathbf{R}_I} E^{\overline{\text{QM}}}(R_{\text{slab}})$ during each time step of the velocity Verlet integrator[18] employed in the latter by means of an external periodic DFT code. Adaption to arbitrary such codes is simple, since the QM/Me approach

published in *Angew. Chem. Int. Ed.* **2014**, *53*, 4721–4724, DOI: 10.1002/anie.201400066

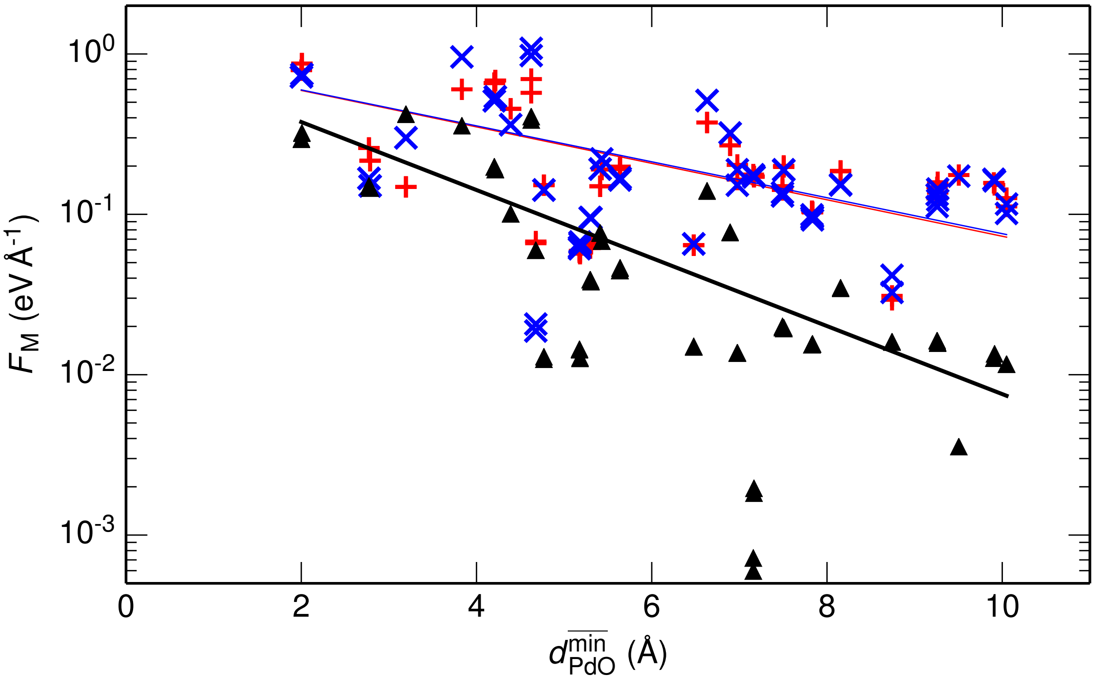


***Figure 3:*** (color online). Decay of forces $F_M$ acting on metal atoms within QM/Me with increasing minimal distance $d_{\overline{\text{PdO}}}^{\text{min}}$ from the adsorbates. Results shown are for the snapshot displayed in Figure 1 of the main article, with equivalent trends also found for all other steps along the trajectory. Compared are the forces resulting from $E^{\overline{\text{QM}}}(R_{\text{slab}} \cup R_{\text{ads}})$ (red plusses) and $E^{\overline{\text{QM}}}(R_{\text{slab}})$ (blue crosses) of the two QM calculations with the force differences $F_M^{\Delta\overline{\text{QM}}}$ (black triangles) as defined in Equation (1) of the main article. The drawn straight lines are only meant to guide the eye and are based on a least squares fit of $\exp(-\alpha\, d_{\overline{\text{PdO}}}^{\text{min}})$. Notwithstanding, it is noteworthy that the decay constant $\alpha$ for the force differences $F_M^{\Delta\overline{\text{QM}}}$ (black triangles) is about twice as large as the almost identical two for the QM forces.

does not require any modifications of the former. This is similar to what is usually termed *mechanical embedding* in conventional QM/MM embedding, but an important difference compared to approaches relying on an electronic embedding potential.[19,20] A simple but robust file and script based mechanism is used for the forward and backward communication of the two coordinate and force sets, respectively. At present, more details about this implementation can be found in the appendix of the main author's PhD thesis.[7]

Figure 3 quantifies the effective separation of short-ranged chemical and long-ranged elastic interactions achieved in QM/Me by comparing the decay of direct QM forces and their force difference with increasing minimal distance $d_{\overline{\text{PdO}}}^{\text{min}}$ in the embedding cell (with positions $R_{\text{slab}}$) from

the adsorbates (with positions $R_{\text{ads}}$). This distance is defined by

$$d_{\text{PdO}}^{\overline{\text{min}}} = \min_{\mathbf{R}_J \in R_{\text{ads}}} \min_{\mathbf{R}_I \in \overline{R_{\text{slab}}}} |\mathbf{R}_I - \mathbf{R}_J| \quad . \tag{4}$$

Here $\overline{R_{\text{Me}}}$ includes all periodic images according to the periodic boundary conditions used in the DFT slab calculations, so that $d_{\text{PdO}}^{\overline{\text{min}}}$ is defined in accordance with the usual minimum image convention. For the embedding cell consisting of a $8 \times 3$ multiple of the Pd(100) surface unit cell with 3 layers employed for the trajectories presented here, the force components on most distant atoms have decayed to about $\leq 10^{-2}$ eVÅ$^{-1}$. This is less than what is often afforded in *ab initio* molecular dynamics (AIMD) trajectories of when fitting CIPs. Of course, the size of the embedding cell is a crucial but well controllable parameter for QM/Me simulations. We have verified that in particular the maximum oxygen-oxygen separation distance shown in Figure 2 (b) is converged with respect to the latter. A detailed assessment can be found in the main author's PhD thesis [7] and will be published elsewhere.

Figure 4 shows the quality of the energy conservation within the employed computational setup. Note that the same implementation of the Velocity verlet integrator as provided by LAMMPS has been used in all three cases. Smaller time steps than $\Delta t = 2.5$ fs do not to yield any improvements. Consequently, the variation of $E_{\text{tot}}$ by less than 2 meV per atom is not related to time discretization during the integration. For the two conventional AIMD trajectories with both the mobile and frozen slab substrate numerical inaccuracies in the DFT forces are thus the obvious culprit. [10,11] In fact, without the special care described in Section 2 above, the corresponding errors have even been significantly larger. In case of QM/Me, force contributions from the MEAM potential could further impair the energy conservation quality. However, these contributions are analytically exact in the LAMMPS implementation, and $\Delta t = 2.5$ fs is relatively small on a phononic time scale, i.e. for the motion of metal atoms (in the bath). They do not significantly contribute to the variation of $E_{\text{tot}}$ therefore, which has also been corroborated by simulation of a slightly heated MEAM bath without any embedding. Altogether, the total energy is conserved with the same

published in *Angew. Chem. Int. Ed.* **2014**, *53*, 4721–4724, DOI: 10.1002/anie.201400066

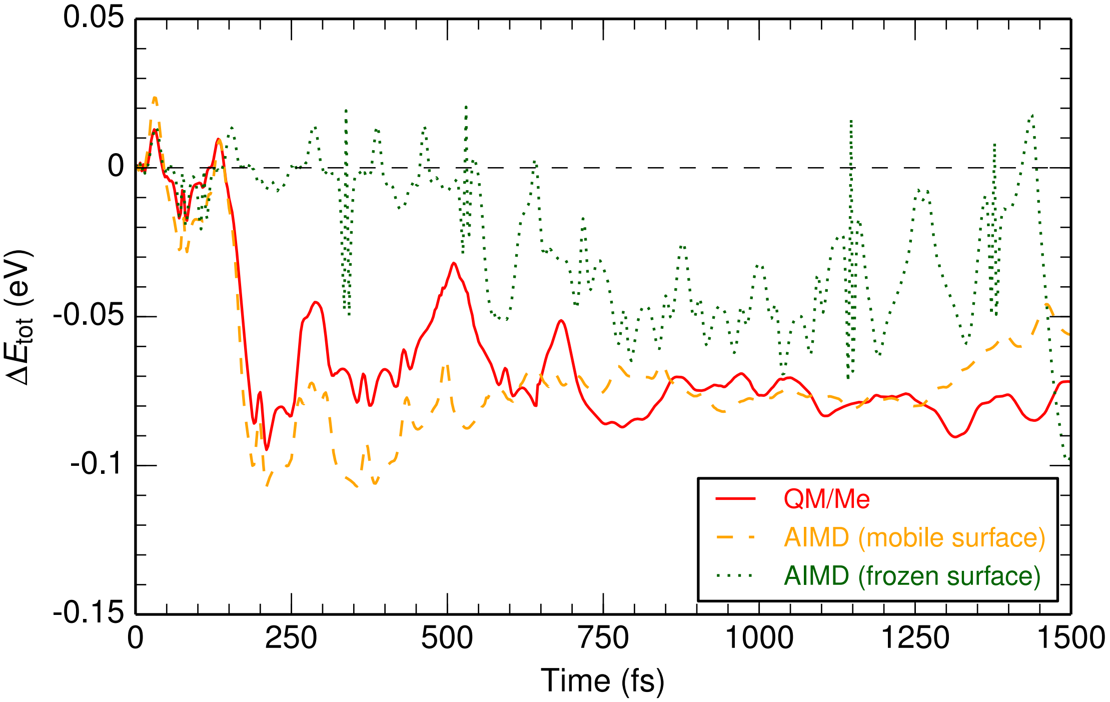


***Figure 4:*** Change of the total energy $E_{tot}$ relative to the initial time step during the MD trajectories also discussed in the main article. The same coloring as in Figure 2 of the latter is used. Note that the absolute value for $E_{tot}$ is shown here, not the frequently given change per atom.

published in *Angew. Chem. Int. Ed.* **2014**, *53*, 4721–4724, DOI: 10.1002/anie.201400066

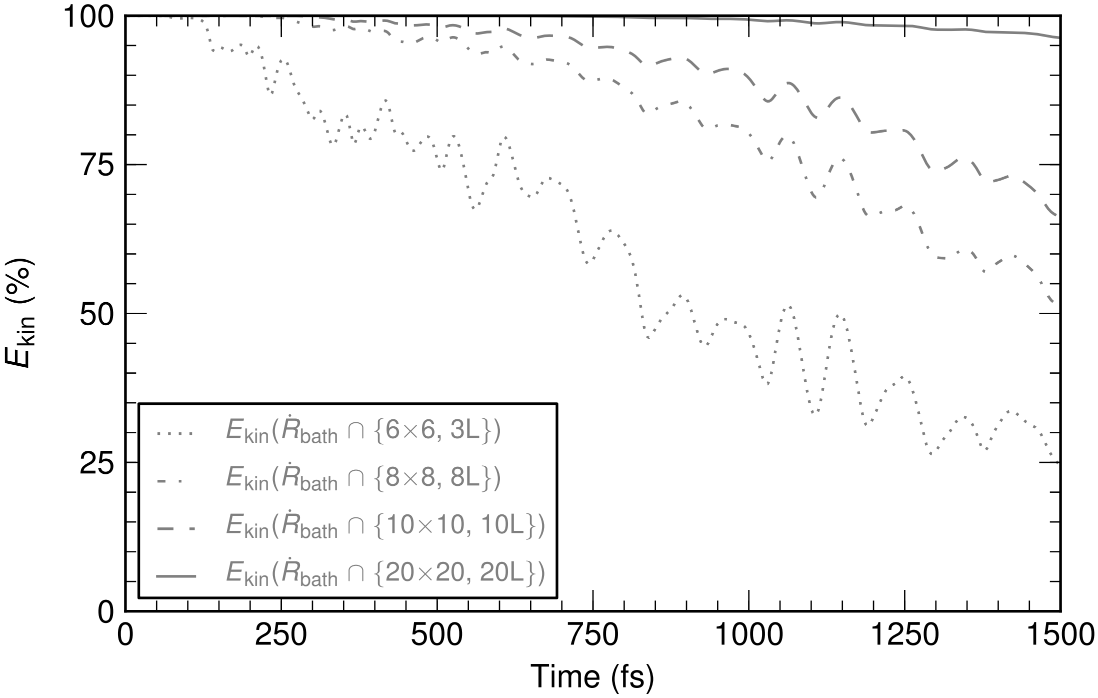


***Figure 5:*** Percentage of the total kinetic energy of the bath $E_{kin}(\dot{R}_{bath})$ contained in $X \times Y$ supercells with $Z$ layers centered around the impingement point of the $O_2$ molecule as indicated by $R_{bath} \cap \{X \times Y, Z\text{L}\}$ in the legend.

quality for the QM/Me as for the AIMD trajectories. This numerically verifies that QM/Me indeed yields a conserved quantity

$$E_{\text{tot}} = \underbrace{\frac{1}{2}\sum_{I\in R} m_I \dot{\mathbf{R}}_I^2}_{E_{\text{kin}}} + V^{\text{QM/Me}} \tag{5}$$

when the resulting forces given by Equations (2) and (3) are employed, and also validates the present implementation. We note that this holds for any size of the embedding cell, as we have explicitly confirmed by using $6\times4$ slabs with 4 layers and $10\times3$ slabs with 3 layers. The systematic embedding-induced errors indicated in the previous paragraph have thus to be clearly distinguished from the numerical force DFT-convergence-errors discussed here.

Unlike for the "small" embedding cell, the periodic boundary conditions which have been chosen for the bath in lateral directions for the sake of convenience, do not affect the simulation: as confirmed by Figure 5, sufficiently many Pd atoms have been included in the bath so that phonon

propagation has not yet reached its periodic boundaries on the time scale considered here. A crude *a priori* estimate of the required bath size can actually be made based on the speed of sound in bulk Pd $v_{\mathrm{sound}}^{\mathrm{Pd}} \approx 31$ Å/ps[21] plus generously (and literally) adding some "safety margin". Since the DFT calculations dominate the computational effort by far (i.e. on the order of minutes are required per time step), ten to hundred times more bath atoms can easily be included without the evaluation of $V^{\mathrm{Me}}$ becoming the bottleneck – or even more when exploiting parallelism (typically with linear scaling) for the latter. On the other hand, modeling even the minimal bath size deduced from Figure 5 $(20 \times 20, 20L)$ entirely within DFT would be more than five orders of magnitude more expensive according to the recent comparison of Plimpton and Thompson.[17] Even if linear scaling DFT approaches should become largely available for metallic systems, this will be impossible in a dynamical (not even to mention statistical) context. Consequently, only our QM/Me embedding approach can enable to tackle problems of similar size and accuracy demands in the foreseeable future.

# References


[1] S. Plimpton, *J. Comput. Phys.* **1995**, *117*, 1 – 19.

[2] S. J. Clark, M. D. Segall, C. J. Pickard, P. J. Hasnip, M. I. J. Probert, K. Refson, M. C. Payne, *Z. Kristallogr.* **2009**, *220*, 567 – 570.

[3] M. I. Baskes, *Phys. Rev. B* **1992**, *46*, 2727 – 2742.

[4] H. J. Monkhorst, J. D. Pack, *Phys. Rev. B* **1976**, *13*, 5188 – 5192.

[5] M. Methfessel, A. T. Paxton, *Phys. Rev. B* **1989**, *40*, 3616 – 3621.

[6] J. P. Perdew, K. Burke, M. Ernzerhof, *Phys. Rev. Lett.* **1996**, *77*, 3865 – 3868.

[7] J. Meyer, PhD thesis, Freie Universität Berlin, **2012**.

[8] J. Meyer, K. Reuter, *New J. Phys.* **2011**, *13*, 085010.

[9] N. Marzari, D. Vanderbilt, M. C. Payne, *Phys. Rev. Lett.* **1997**, *79*, 1337 – 1340.

[10] J. M. Herbert, M. Head-Gordon, *Phys. Chem. Chem. Phys.* **2005**, *7*, 3269 – 3275.

[11] A. M. N. Niklasson, *Phys. Rev. Lett.* **2008**, *100*, 123004.

[12] P. van Beurden, G. J. Kramer, *Phys. Rev. B* **2001**, *63*, 165106.

[13] F. Ercolessi, J. B. Adams, *Europhys. Lett.* **1994**, *26*, 583.

[14] S. M. Valone, M. I. Baskes, R. L. Martin, *Phys. Rev. B* **2006**, *73*, 214209.

[15] J. Behler, M. Parrinello, *Phys. Rev. Lett.* **2007**, *98*, 146401.

[16] A. P. Bartók, M. C. Payne, R. Kondor, G. Csányi, *Phys. Rev. Lett.* **2010**, *104*, 136403.

[17] S. M. Foiles, M. I. Baskes, *MRS Bulletin* **2012**, *37*, 485–491.

[18] W. C. Swope, H. C. Andersen, P. H. Berens, K. R. Wilson, *J. Chem. Phys.* **1982**, *76*, 637 – 649.

[19] N. Choly, G. Lu, W. E, E. Kaxiras, *Phys. Rev. B* **2005**, *71*, 094101.

[20] X. Zhang, Q. Peng, G. Lu, *Phys. Rev. B* **2010**, *82*, 134120.

[21] *Handbook of the physicochemical properties of the elements*, (Ed.: G. V. Samsonov), IFI/Plenum, **1968**.
